# Supplementary material for: Quantitative Information Extraction from Humanitarian Documents
Source: arXiv:2408.04941 source file (2024-08-09)
Supplement: Supplementary file 1 [file annotation_schema.pdf]

# Annotation schema

The six following tags represent our annotation schema:

- Number
- Unit
- Modifier
- EventP
- EventA
- EventO

First, find a *Number* and then annotate other tags around it, if any (do **not** annotate all the other tags if there is no *Number* in a phrase!).

The *Number* is an explicit numeral. If the *Number* is linked to an *EventX* this tuple is considered a quantity, so something relevant to a humanitarian event dealing with people, aid, or any other activity that is related to humanitarian action, otherwise it is just a raw number.

Ideally, each annotated quantity would have at a minimum a *Number*, *Unit* to which it refers, and an *EventX* that explains what happened to that *Number* of *Unit* s.

All tags in a phrase are then connected with arrows, each arrow originating from *Number*.

Some text can be tagged with multiple labels (often a unit can also be a signifier of an event).

**Example:**

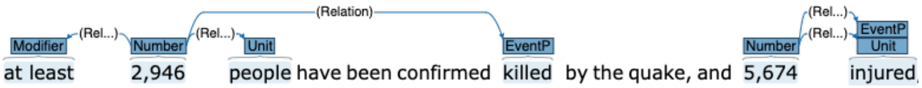


## Number

- Any explicit numeral (as defined on UniversalDependencies), expressed by letters, digits or a combination of both.
- *Number* could be money, percentages, supplies, places, years, distances, etc., but it is **not** dates, page numbers, section numbers or report numbers.
- If the annotated number is a percentage, annotate the `%` symbol or the `percent` word too (e.g. **10 per cent** of people, **5%** of them, etc.).
- Do not tag numbers that are part of a proper noun (e.g. “Camp 3”).

- Tag only explicit numerical values, do not tag words like “a”, “an”, “many” and “a lot”.

**Examples**

- **800 million** people
- around **one million** women
- a **thousand** refugees
- around **200** people out of **400** need assistance
- **50%** of the displaced people (i.e. **200** out of **400** people) need help
- **100** people are missing since August, 3rd
- the government provided **50,000** USD to support the population
- the average age was **70** years

---

## Modifier

- Only used for terms like “over”, “about” or “on average” that modify a *Number*.
- Signify a relation by dragging an arrow from *Number* to *Modifier*.

**Examples**

- **over** 800 displaced people
- **about** 1 million girls
- the **median number** is 50 people
- the amount **ranges** from 10 to 20 cases

---

## Unit

- The unit is the thing or things a *Number* refers to.
- These are often people, but can be objects or places.
- Do not annotate pronouns as *Unit*, but what it references.
- If the unit is made of several conjuncted words, tag all of them as a single *Unit*.
- Some *Units* can be “fatalities” or “deaths”, as they imply “people” with additional information.
- Include modifiers (e.g. “pregnant” in “pregnant women”) in *Unit*.
- Signify a relation by dragging an arrow from *Number* to *Unit*.

**Examples**

- 800 million **people**
- a hundred **tents** needed
- 1500 **people** displaced, 1000 of whom in need of health assistance

- 300 are **women and girls**
- 100 **pregnant women** need medical assistance
- 20 **tons of supplies** provided
- the government provided 50,000 **USD** to support the population

---

## EventP, EventA and EventO

Only for the _Number_s you find, also annotate the event relevant to it. There are 3 kinds of events tags:

1. EventP: deals with an individual or a group of **P**eople (e.g. around 100 **dengue deaths** were **reported**).
2. EventA: deals with supplies or **A**ssistance that directly affects people (e.g. 300 medical kits **have been supplied**).
3. EventO: deals with something that is not considered by either *EventP* or *EventA* or when it is difficult to distinguish between the two (e.g. the organization **surveyed** six households).

- A sentence may have more than one event relevant to a number, annotate all of them.
- Some text can be both an event and a unit, tag it with both the labels ("dengue deaths").
- Select the smallest meaningful piece of text capable of describing the event itself plus all the modifiers that can add more details to it.
- We are not interested in what caused the problem (e.g. a storm, an earthquake), we are interested, instead, in the status of the affected people (e.g. displaced, dead, in need of assistance).
- In some cases the event can be expressed with words that are not verbs but nouns or adjectives (e.g. "death toll" for death or "unaccounted for" for displacement).
- Signify a relation by dragging an arrow from *Number* to the event.

**Examples**

- 100 people in **need of lifesaving devices**
- 1 thousand **internally displaced** people
- 800 women are in **urgent need of health assistance**
- people in **need of health assistance and basic supplies**
- 800 civilian **deaths**
- 1000 **fatalities** (in this case the annotator can be unsure if is a unit or an event, so it will be tagged with both labels)
